# Supplementary material for: A Universal Density Matrix Functional from Molecular Orbital-Based Machine Learning: Transferability across Organic Molecules
Source: arXiv:1901.03309 ancillary file (2019-04-04)
Supplement: Supplementary file 1 [file si.pdf]

# Supporting Information for A Universal Density Matrix Functional from Molecular Orbital-Based Machine Learning: Transferability across Organic Molecules

Lixue Cheng and Matthew Welborn
*Division of Chemistry and Chemical Engineering,*
*California Institute of Technology, Pasadena, CA 91125, USA*

Anders S. Christensen
*Institute of Physical Chemistry and National Center for Computational Design and Discovery of Novel Materials,*
*Department of Chemistry, University of Basel, Basel, Switzerland*

Thomas F. Miller III
*Division of Chemistry and Chemical Engineering,*
*California Institute of Technology, Pasadena, CA 91125, USA, tfm@caltech.edu*
(Dated: April 4, 2019)

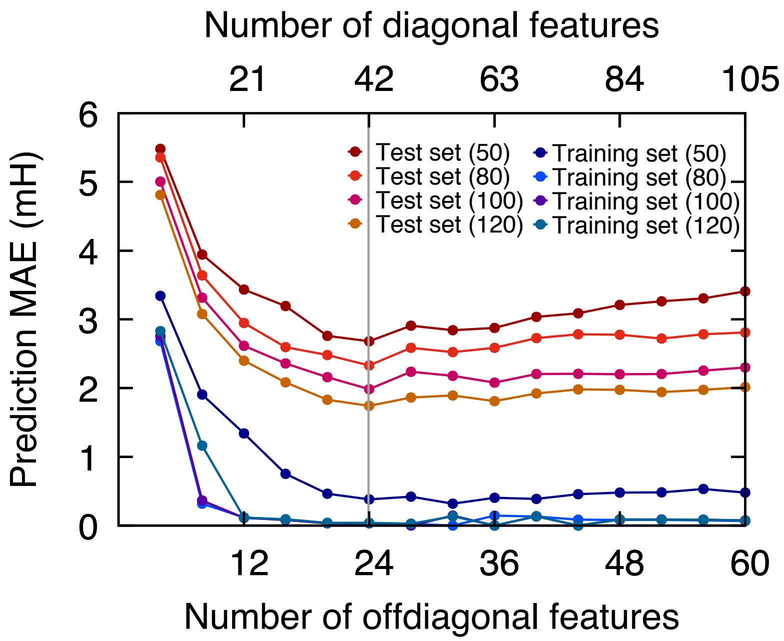


FIG. S1. Prediction MAE for MOB-ML models trained on the QM7b-T dataset as a function of the number of MOB-ML features selected. Predictions are made for the training set and for a test set comprised of the remainder of QM7b-T, with the number of molecules included in the training set indicated in parentheses. Features are included in order of decreasing RFR-MDA importance. The gray line indicates the number of features employed for training on the QM7b-T dataset in the main text (Fig. 3); here, the ratio of the number of diagonal features to off-diagonal features is fixed at 42:24. Regardless of whether the MOB-ML models are trained using either 50, 80, 100 and 120 molecules, the accuracy of the test-set prediction is relatively insensitive to the number of selected MOB-ML features.

TABLE S1. MAE and MAE/heavy atom of MOB-ML on predicting QM7b-T and GDB-13-T using a model trained on QM7b-T (energies in mH).

| | QM7b-T, MP2/cc-pVTZ | | QM7b-T, CCSD(T)/cc-pVDZ | | GDB-13-T, MP2/cc-pVTZ | |
|---|---|---|---|---|---|---|
| Training set size | MAE | MAE/heavy atom | MAE | MAE/heavy atom | MAE | MAE/heavy atom |
| 20 | 4.536 | 0.6664 | 4.962 | 0.7314 | 8.711 | 0.6701 |
| 30 | 3.966 | 0.5844 | 3.865 | 0.5690 | 7.554 | 0.5811 |
| 40 | 3.183 | 0.4696 | 3.605 | 0.5309 | 5.731 | 0.4408 |
| 50 | 2.938 | 0.4338 | 3.180 | 0.4678 | 5.375 | 0.4135 |
| 60 | 2.774 | 0.4094 | 2.960 | 0.4371 | 5.020 | 0.3862 |
| 70 | 2.660 | 0.3906 | 2.540 | 0.3751 | 5.055 | 0.3888 |
| 80 | 2.519 | 0.3701 | 2.538 | 0.3755 | 4.669 | 0.3591 |
| 90 | 2.165 | 0.3116 | 2.266 | 0.3354 | 4.161 | 0.3201 |
| 100 | 2.085 | 0.3076 | 2.187 | 0.3235 | 4.150 | 0.3192 |
| 110 | 1.878 | 0.2768 | 2.037 | 0.3017 | 3.880 | 0.2985 |
| 120 | 1.797 | 0.2650 | 2.040 | 0.3023 | 3.809 | 0.2930 |
| 130 | 1.747 | 0.2582 | 2.013 | 0.2987 | 3.746 | 0.2882 |
| 140 | 1.681 | 0.2484 | 1.967 | 0.2921 | 3.692 | 0.2840 |
| 150 | 1.674 | 0.2475 | 1.998 | 0.2962 | 3.665 | 0.2820 |
| 160 | 1.645 | 0.2429 | 1.921 | 0.2855 | 3.654 | 0.2810 |
| 170 | 1.620 | 0.2394 | 1.911 | 0.2834 | 3.652 | 0.2809 |
| 180 | 1.577 | 0.2333 | 1.865 | 0.2778 | 3.611 | 0.2778 |
| 190 | 1.511 | 0.2240 | 1.827 | 0.2728 | 3.592 | 0.2763 |
| 200 | 1.511 | 0.2244 | 1.802 | 0.2696 | 3.605 | 0.2773 |
| 210 | 1.443 | 0.2140 | 1.801 | 0.2696 | 3.607 | 0.2774 |
| 220 | 1.427 | 0.2115 | 1.802 | 0.2698 | 3.617 | 0.2782 |

TABLE S2. MAE of FCHL/Δ-ML on predicting QM7b-T and GDB-13-T using a model trained on QM7b-T (energies in mH). The standard error of the mean (SEM) over 10 trials is also reported.

| | QM7b-T, MP2/cc-pVTZ | | GDB-13-T, MP2/cc-pVTZ | | | |
|---|---|---|---|---|---|---|
| Training set size | MAE | SEM | MAE | SEM | MAE/heavy atom | SEM/heavy atom |
| 1 | 227.7 | 16.94 | 444.4 | 44.37 | 34.18 | 3.413 |
| 2 | 120.5 | 16.38 | 212.3 | 35.36 | 16.33 | 2.720 |
| 3 | 94.65 | 24.05 | 169.4 | 32.20 | 13.03 | 2.477 |
| 4 | 51.88 | 9.660 | 115.1 | 20.51 | 8.857 | 1.578 |
| 5 | 34.99 | 4.574 | 78.56 | 11.20 | 6.043 | 0.8618 |
| 6 | 20.37 | 1.943 | 56.29 | 5.873 | 4.330 | 0.4518 |
| 7 | 23.07 | 3.799 | 51.16 | 8.810 | 3.935 | 0.6777 |
| 8 | 19.04 | 1.639 | 42.21 | 5.878 | 3.247 | 0.4521 |
| 9 | 19.23 | 1.975 | 43.06 | 8.492 | 3.313 | 0.6532 |
| 10 | 14.22 | 1.671 | 43.05 | 6.783 | 3.312 | 0.5217 |
| 20 | 7.823 | 0.5624 | 22.80 | 2.744 | 1.754 | 0.2111 |
| 30 | 6.501 | 0.5400 | 17.72 | 2.161 | 1.363 | 0.1663 |
| 40 | 5.219 | 0.1874 | 15.87 | 1.477 | 1.221 | 0.1136 |
| 50 | 4.567 | 0.2395 | 13.64 | 1.549 | 1.049 | 0.1192 |
| 60 | 3.887 | 0.1713 | 11.57 | 0.6267 | 0.8897 | 0.04821 |
| 70 | 3.889 | 0.1453 | 10.11 | 0.9725 | 0.7780 | 0.07480 |
| 80 | 3.608 | 0.2412 | 9.704 | 1.311 | 0.7465 | 0.1008 |
| 90 | 3.283 | 0.1016 | 9.062 | 0.6463 | 0.6971 | 0.04971 |
| 100 | 3.205 | 0.08087 | 8.787 | 0.7807 | 0.6759 | 0.06006 |
| 200 | 2.396 | 0.03973 | 7.265 | 0.5289 | 0.5588 | 0.04068 |
| 300 | 2.022 | 0.03468 | 5.722 | 0.2212 | 0.4401 | 0.01701 |
| 400 | 1.870 | 0.01906 | 5.706 | 0.2140 | 0.4389 | 0.01646 |
| 500 | 1.760 | 0.02530 | 5.615 | 0.6035 | 0.4319 | 0.04642 |
| 600 | 1.648 | 0.01538 | 5.128 | 0.2007 | 0.3945 | 0.01544 |
| 700 | 1.581 | 0.02471 | 4.946 | 0.1344 | 0.3805 | 0.01034 |
| 800 | 1.503 | 0.02184 | 5.140 | 0.3127 | 0.3954 | 0.02405 |
| 900 | 1.445 | 0.01963 | 5.134 | 0.2843 | 0.3949 | 0.02187 |
| 1000 | 1.408 | 0.02135 | 5.584 | 0.5120 | 0.4295 | 0.03938 |
| 2000 | 1.135 | 0.01120 | 4.626 | 0.1944 | 0.3559 | 0.01495 |
| 3000 | 0.9837 | 0.003951 | 4.094 | 0.1812 | 0.3149 | 0.01394 |
| 4000 | 0.8995 | 0.006155 | 3.816 | 0.1211 | 0.2935 | 0.00931 |
| 5000 | 0.8618 | 0.005251 | 3.865 | 0.1691 | 0.2973 | 0.01301 |
